# Supplementary material for: The Benefits of Reusing Batches for Gradient Descent in Two-Layer Networks: Breaking the Curse of Information and Leap Exponents
Source: arXiv:2402.03220 source file (2024-06-30)
Supplement: Supplementary file 1 [file DMFT.tex]

\section{DMFT derivation}
\label{sec:app:dmft}
This section will have marginally different notations, mostly because of the different scaling needed in the computation. This is a technical detail and it's possible to show that these convenctions from here onward are equivalent to the ones above.

Consider a dataset $\{\bf x_{\nu},y_{\nu}\}_{\nu=1,...,n}$ with $n$ points, each of dimension $d$, with $\bf x_{\nu} \in \mathbb{R}^d$. 
We have a simple Gaussian input $\bf x_{\nu} \sim \mathcal{N}(0,\mathbf{1}_{d\times d})$, where the labels are generated by a two-layer teacher with $K_T$ weights ${\bf w^{\star}}^k \sim \mathcal{N}(0,\mathbf{1}_{d\times d})$ in the first layer and one ${\bf u^\star} = \mathbb{R}^{K_T}$ set of weights in the second layer. We will start with a generic computation in which we also learn the second layer, and we will make it constant when it will be convenient to us. The teacher will have non-linearity $\phi_{T}:\mathbb{R}\to\mathbb{R}$:
$$
    y_\nu = \frac{1}{\sqrt{K_T}}\sum_{k=1}^{K_T} u_k^\star \phi_{T}\left(\frac{{ {{\bf w^{\star}}}^k}^\top \bf x_\nu}{\sqrt{d}}\right)
$$
We are in the $d\to\infty$, $n\to\infty$ limit, with $K_T$ fixed.
We again define the risk $\mathcal{R}(\bf w)$:
\begin{equation}
    \mathcal{R}({\bf w}) = \frac{\lambda_U}{2}\Vert{\bf u}\Vert_2 ^2 + \frac{\lambda_W}{2}\Vert{\bf w}\Vert_2 ^2 + \sum_{\nu=1}^n \mathcal{L} \left( y_{\nu}, \frac{1}{\sqrt{K_S}}\sum_{k=1}^{K_S} u_k \phi_{S}\left(\frac{{ {{\bf w}}^k}^\top \bf x_\nu}{\sqrt{d}}\right)\right)
\end{equation}
Using gradient descent we get two differential equations:

\begin{equation}
\begin{split}
{\bf w}_{t+1}=&{\bf w}_t -\eta\left[\lambda_W {\bf w}_t +\sum_{\nu=1}^n \,\frac{\partial \mathcal{L}}{\partial {\bf w}_t}\left(y_{\nu}, \frac{1}{\sqrt{K_S}}\sum_{k=1}^{K_S} u_{k,t} \phi_{S}\left(\frac{{{\bf w}_t^k}^\top \bf x_\nu}{\sqrt{d}}\right)\right)  \right]   \\
{\bf u}_{t+1}=&{\bf u}_t -\eta\left[\lambda_U {\bf u}_t +\sum_{\nu=1}^n \,\frac{\partial \mathcal{L}}{\partial {\bf u}_t}\left(y_{\nu}, \frac{1}{\sqrt{K_S}}\sum_{k=1}^{K_S} u_{k,t} \phi_{S}\left(\frac{{{\bf w}_t^k}^\top \bf x_\nu}{\sqrt{d}}\right)\right)  \right]   
\end{split}
\end{equation}

We need a Grassman trick to write this using Grassman variables. First, define:
\begin{equation}
    {\bf w}(a)={\bf w}(t_a)+\theta_a \bar{\theta}_a  {\bf \hat{w}}(t_a)\,,\qquad\qquad {\bf u}(a)={\bf u}(t_a)+\theta_a \bar{\theta}_a  {\bf \hat{u}}(t_a).
\end{equation}
Then notice that for any function $f(\cdot, \cdot)$ the following identity:

\begin{equation}
\int \text{d} a \,f \left({\bf w}(a),{\bf u}(a)\right) = \int_0^{+\infty} \text{d} t_a {\bf \hat{w}}(t_a)^\top \frac{\partial f}{\partial {\bf w}}\left({\bf w}(t_a),{\bf u}(t_a)\right) + {\bf \hat{u}}(t_a)^\top \frac{\partial f}{\partial {\bf u}}\left({\bf w}(t_a),{\bf u}(t_a)\right)
\end{equation}
The proof is entirely analogous to the one-layer one. We thus have a dynamical partition function:

\begin{equation}
1 = Z_{\rm dyn} = \left\langle\int \mathcal{D}{\bf w}\mathcal{D}{\bf \hat w}\mathcal{D}{\bf u}\mathcal{D}{\bf \hat u} \,e^{S_{\rm dyn}}\right\rangle
\end{equation}
with:

\begin{equation}
\begin{split}
S_{\rm dyn} = -\sum_{k=1}^{K_S}\frac{1}{2} \int \text{d} a \text{d} b\, \mathcal{K}_W(a,b) {{\bf w}^k}(a)^\top {{\bf w}^k}(b)-\frac{1}{2} \int \text{d} a \text{d} b\, \mathcal{K}_U(a,b) {\bf u}(a)^\top {\bf u}(b)-\\-\sum_{\nu=1}^n\int \text{d} a\, \mathcal{L}\left( \frac{1}{\sqrt{K_T}}\sum_{k=1}^{K_T} u_k^\star \phi_{T}\left(\frac{{ {{\bf w^{\star}}}^k}^\top \bf x_\nu}{\sqrt{d}}\right), \frac{1}{\sqrt{K_S}}\sum_{k=1}^{K_S} u_k (a)\phi_{S}\left(\frac{{{\bf w}(a)^k}^\top \bf x_\nu}{\sqrt{d}}\right)\right)    
\end{split}
\end{equation}
We define the pre-activation variables on the first layer ${\bf h}_\nu(a)$ and ${\bf h}^\star_\nu$:

\begin{equation}
    h_\nu^k(a) = \frac{{\bf w}^k(a)\top {\bf x}_{\nu}}{\sqrt{d}}, \qquad\qquad {h^k_\nu}^\star = \frac{{{{\bf w}
    ^\star}^k}^\top {\bf x}_{\nu}} {\sqrt{d}}
\end{equation}
With this substitution the action becomes:

\begin{equation}
\begin{split}
S_{\rm dyn} = -\sum_{k=1}^{K_S}\frac{1}{2} \int \text{d} a \text{d} b\, \mathcal{K}_W(a,b) {{\bf w}^k}(a)^\top {{\bf w}^k}(b)-\frac{1}{2} \int \text{d} a \text{d} b\, \mathcal{K}_U(a,b) {\bf u}(a)^\top {\bf u}(b)-\\-\sum_{\nu=1}^n\int \text{d} a\, \mathcal{L}\left( \frac{{{\bf u}^\star}^\top \phi_{T}({\bf h}^\star_\nu)}{\sqrt{K_T}} , \frac{{\bf u} (a)^\top\phi_{S}({\bf h}_\nu(a))}{\sqrt{K_S}}\right)    
\end{split}
\end{equation}
Of course these new definitions will force us to introduce Lagrange multipliers $\hat {\bf h}^\star_\nu$ and $\hat {\bf h}_\nu$. This will result in an additional entropic term in the action:

\begin{equation}
    \sum_{\nu=1}^n\left[\int \text{d} a \, \sum_{k=1}^{K_S}\, \hat{\bf h}_{\nu}^k(a)\left(h_{\nu}^k(a)-\frac{{\bf w}^k(a)^\top {\bf x}_{\nu}}{\sqrt{d}}\right) + \sum_{k=1}^{K_T}\, {h^k_\nu}^\star\left({h^k_{\nu}}^\star-\frac{{{\bf w}^\star}^\top {\bf x}_{\nu}}{\sqrt{d}}\right)\right]
\end{equation}
We now do a bit of rewriting in order to average over the data:

\begin{equation}
\begin{split}
    & \sum_{\nu=1}^n\left[\sum_{k=1}^{K_S}\int \text{d} a \, \hat{\bf h}_{\nu}^k(a)\left(h_{\nu}^k(a)-\frac{{\bf w}^k(a)^\top {\bf x}_{\nu}}{\sqrt{d}}\right) + \sum_{k=1}^{K_T}\, {h^k_\nu}^\star\left({h^k_{\nu}}^\star-\frac{{{\bf w}^\star}^\top {\bf x}_{\nu}}{\sqrt{d}}\right)\right]\\
    =&\sum_{\nu=1}^n\left[\int \text{d} a \, \hat{{\bf h}}_{\nu}(a)^\top{\bf h}_{\nu}(a) + \hat{{\bf h}}_{\nu}^{\star\top} {\bf h}_{\nu}^\star\right] - \sum_{\nu=1}^n\frac{{\bf x}^\top_{\nu}}{\sqrt{d}}\left[\sum_{k=1}^{K_S}\int \text{d} a \, \hat{\bf h}_{\nu}^k(a){\bf w}^k(a) + \sum_{k=1}^{K_T}\hat{\bf h}_{\nu}^{k\star}{\bf w}^{k\star}\right]\\
\end{split}
\end{equation}
Averaging over the Gaussian input ${\bf x}_\nu$ we obtain:

\begin{equation}
\begin{split}
    \sum_{\nu=1}^n\left[\int \text{d} a \, \hat{{\bf h}}_{\nu}(a)^\top{\bf h}_{\nu}(a) + \hat{{\bf h}}_{\nu}^{\star\top} {\bf h}_{\nu}^\star +\frac{1}{2} \int\text{d}a\text{d}b\,\hat{{\bf h}}_{\nu}(a)^\top {\bf Q}_W(a,b)\hat{\bf h}_{\nu}(a) \right.\\\left.
    +\frac{1}{2} \hat{{\bf h}}_{\nu}^{\star\top}\hat{\bf h}_{\nu}^\star + \int\text{d}a\,\hat{{\bf h}}_{\nu}(a)^\top {\bf m}_W(a)\hat{\bf h}_{\nu}^\star\right] 
\end{split}
\end{equation}
where we introduced the order parameters ${\bf m}_W(a)$ and ${\bf Q}_W(a,b)$:

\begin{equation}
    m^{k_1k_2}_W(a)=\frac{{\bf w}^{k_1}(a)^\top {\bf w}^{k_2}\star}{d}, \qquad Q^{k_1k_2}_W(a,b)=\frac{{\bf w}^{k_1}(a)^\top{\bf w}^{k_2}(b)}{d}
\end{equation}
Terms with different $\nu$ will be decoupled, so we drop the $\nu$. The new definitions will induce an entropic term:

\begin{equation}
\begin{split}
    &d\int \text{d}a \, {\rm Tr}\left[\hat {\bf m}_W(a)^\top {\bf m}_W(a)\right] + d\int \text{d}a\text{d}b\, {\rm Tr}\left[\hat {\bf Q}_W(a,b)^\top {\bf Q}_W(a,b)\right]+\\ &\qquad\qquad\qquad\qquad + \sum_{i=1}^d \left(-\int \text{d}a \,{\bf w}_i(a)^\top \hat{\bf m}_W(a){\bf w}_i^\star - \int \text{d}a\text{d}b\, {\bf w}_i(a)^\top \hat{\bf Q}_W(a,b){\bf w}_i(a) \right)
\end{split}
\end{equation}
Integrating over each ${\bf w}_i$ we get:

\begin{equation}
    -\frac{d}{2}\log{\det{(2\hat{\bf Q}_W (a,b))}} + \sum_{i=1}^d\sum_{k_1,k_2}^{K_T}\sum_{h_1,h_2}^{K_S}\frac{{\rm w}_i^{h_1\star}{\rm w}_i^{h_2\star}}{4} \int \text{d}a \text{d}b \,\hat m_W^{k_1h_1} (a)({\hat{Q}_W}^{-1})^{k_1k_2}(a,b)\hat m_W^{k_2h_2} (b)  
\end{equation}
By concentration of ${\bf w}^\star_i$ we have:

\begin{equation}
    -\frac{d}{2}\log{\det{(2\hat{\bf Q}_W (a,b))}} + \sum_{h}^{K_S}\sum_{k_1,k_2}^{K_T}\frac{d}{4} \int \text{d}a \text{d}b \,\hat m_W^{k_1h} (a)({\hat{Q}_W}^{-1})^{k_1k_2}(a,b)\hat m_W^{k_2h} (b)  
\end{equation}
For each $h$ this is a Gaussian integral on $\hat m_W$. After integrating we get:

\begin{equation}
    -\frac{d}{2}\log{\det{(2\hat{\bf Q}_W (a,b))}} - \sum_{h}^{K_S}\sum_{k_1,k_2}^{K_T}d \int \text{d}a \text{d}b \,m_W^{k_1h} (a)({\hat{Q}_W})^{k_1k_2}(a,b) m_W^{k_2h} (b)  
\end{equation}
Computing the saddle point on $\hat Q_W$ we get:

\begin{equation}
    ({\hat{Q}_W}^{-1})^{k_1k_2}(a,b) = (Q_W)^{k_1k_2}(a,b) - \sum_{h=1}^{K_S}m_W^{k_1h} (a)m_W^{k_2h} (b)
\end{equation}
Or equivalently:

\begin{equation}
    {\hat{{\bf Q}}_W}^{-1}(a,b) = {{\bf Q}_W}(a,b) - {\bf m}_W (a){{\bf m}_W}^\top (b)
\end{equation}
So the only contribution from these last two overlaps is:

\begin{equation}
    \frac{d}{2}\log{\det{\left({\bf Q}_W (a,b)-{\bf m}_W (a){{\bf m}_W}^\top (b)\right)}}
\end{equation}
The kinetic term for ${\bf w}$ is on the other hand:

\begin{equation}
    -\sum_{k=1}^{K_S}\frac{1}{2} \int \text{d} a \text{d} b\, \mathcal{K}_W(a,b) {{\bf w}^k}(a)^\top {{\bf w}^k}(b) = -\frac{d}{2}\int \text{d}a\text{d}b\, {\rm Tr}\left[{\bf Q}_W(a,b)\right]
\end{equation}
To recapitulate, after a translation ${\bf Q}_W (a,b) \to {\bf Q}_W (a,b)+{\bf m}_W (a){{\bf m}_W}^\top (b)$ the dynamical action is:

\begin{equation}
\begin{split}
S_{\rm dyn} = -\frac{d}{2}\int \text{d}a\text{d}b\, \mathcal{K}(a,b){\rm Tr}\left[{\bf Q}_W (a,b)+{\bf m}_W (a){{\bf m}_W}^\top (b)\right]-\frac{1}{2} \int \text{d} a \text{d} b\, \mathcal{K}_U(a,b) {\bf u}(a)^\top {\bf u}(b)+\\
+\frac{d}{2}\log{\det{\left({\bf Q}_W (a,b)\right)}} + n S_{\rm loc}   
\end{split}
\end{equation}
where:

\begin{equation}
\begin{split}
    S_{\rm loc} = \int \text{d} a \, \hat{{\bf h}}(a)^\top{\bf h}(a) + \hat{{\bf h}}^{\star\top} {\bf h}^\star +\frac{1}{2} \int\text{d}a\text{d}b\,\hat{{\bf h}}(a)^\top {\bf Q}_W(a,b)\hat{\bf h}(b) + \frac{1}{2} \hat{\bf h}^{\star\top}\hat{\bf h}^\star \int \text{d} a\, \mathcal{L}\left( \frac{{{\bf u}^\star}^\top \phi_{T}({\bf h}^\star)}{\sqrt{K_T}} , \frac{{\bf u} (a)^\top\phi_{S}({\bf h}(a))}{\sqrt{K_S}}\right)+\\
    + \int\text{d}a\,\hat{\bf h}(a)^\top {\bf m}_W(a)\hat{\bf h}^\star + \frac{1}{2}\left(\int\text{d}a\,\hat{\bf h}(a)^\top {\bf m}_W(a)\right)^2 
\end{split}
\end{equation}
Notice that $\hat {\bf h}^\star$ is again a Gaussian variable, so we integrate over it and obtain:
\begin{equation}
\begin{split}
    S_{\rm loc} = \int \text{d} a \, \hat{{\bf h}}(a)^\top{\bf h}(a) +\frac{1}{2} \int\text{d}a\text{d}b\,\hat{{\bf h}}(a)^\top {\bf Q}_W(a,b)\hat{\bf h}(b) -\int \text{d} a\, \mathcal{L}\left( \frac{{{\bf u}^\star}^\top \phi_{T}({\bf h}^\star)}{\sqrt{K_T}} , \frac{{\bf u} (a)^\top\phi_{S}({\bf h}(a))}{\sqrt{K_S}}\right)+\\
    + \frac{1}{2}\left(\int\text{d}a\,\hat{\bf h}(a)^\top {\bf m}_W(a)\right)^2 - \frac{1}{2}\left(\int\text{d}a\,\hat{\bf h}(a)^\top {\bf m}_W(a) + {\bf h}^\star\right)^2
\end{split}
\end{equation}
or equivalently:

\begin{equation}
\begin{split}
    S_{\rm loc} = \int \text{d} a \, \hat{{\bf h}}(a)^\top\left({\bf h}(a) - {\bf m}_W(a){\bf h}^\star\right) +\frac{1}{2} \int\text{d}a\text{d}b\,\hat{{\bf h}}(a)^\top {\bf Q}_W(a,b)\hat{\bf h}(b) - \frac{1}{2} {\bf h}^{\star\top}{\bf h}^\star - \int \text{d} a\, \mathcal{L}\left( \frac{{{\bf u}^\star}^\top \phi_{T}({\bf h}^\star)}{\sqrt{K_T}} , \frac{{\bf u} (a)^\top\phi_{S}({\bf h}(a))}{\sqrt{K_S}}\right)
\end{split}
\end{equation}
Out of convenience we shift ${\bf h}(a) \to {\bf h}(a) + {\bf m}_W(a){\bf h}^\star$, getting the expression:

\begin{equation}
\begin{split}
    S_{\rm loc} = \int \text{d} a \, \hat{{\bf h}}(a)^\top{\bf h}(a)+\frac{1}{2} \int\text{d}a\text{d}b\,\hat{{\bf h}}(a)^\top {\bf Q}_W(a,b)\hat{\bf h}(b) - \frac{1}{2} {\bf h}^{\star\top}{\bf h}^\star - \int \text{d} a\, \mathcal{L}\left( \frac{{{\bf u}^\star}^\top \phi_{T}({\bf h}^\star)}{\sqrt{K_T}} , \frac{{\bf u} (a)^\top\phi_{S}({\bf h}(a) + {\bf m}_W(a){\bf h}^\star)}{\sqrt{K_S}}\right)
\end{split}
\end{equation}
Integrating also over $\hat{\bf h}(a)$ we obtain:

\begin{equation}
\begin{split}
    S_{\rm loc} = -\frac{1}{2} \int\text{d}a\text{d}b\,{\bf h}(a)^\top {\bf Q}_W^{-1}(a,b){\bf h}(b) - \frac{1}{2} {\bf h}^{\star\top}{\bf h}^\star - \int \text{d} a\, \mathcal{L}\left( \frac{{{\bf u}^\star}^\top \phi_{T}({\bf h}^\star)}{\sqrt{K_T}} , \frac{{\bf u} (a)^\top\phi_{S}({\bf h}(a) + {\bf m}_W(a){\bf h}^\star)}{\sqrt{K_S}}\right)
\end{split}
\end{equation}

\subsection{Saddle point equations}
From here onwards we drop the $W$ in ${\bf Q}_W$, which will be simply called ${\bf Q}$. Similarly, ${\bf m}_W$ will be called ${\bf m}$. We want to keep the second layer fixed, so we remove the functional integral over ${\bf u}$ and the kinetic piece in the action.
Let's take the saddle point equations with respect to ${\bf m}$ and ${\bf Q}$. We will get respectively

\begin{equation}
    \int \text{d}b \,\mathcal{K}(a,b) {\bf m}(b) = \alpha \frac{\partial Z_{\rm loc}}{\partial {\bf m}(a)}
\end{equation}
and:

\begin{equation}
    {\bf Q}^{-1}(a,b) = \mathcal{K}(a,b) - 2\alpha \frac{\partial Z_{\rm loc}}{\partial {\bf Q}(a,b)}
\end{equation}

Making these expressions explicit is a bit tricky. First, define for any observable $\mathcal{O}({\bf h}, {\bf h}^\star)$ the average $\llangle \mathcal{O} \rrangle$ as:

\begin{equation}
    \llangle \mathcal{O} \rrangle = \int \mathcal{D}{\bf h}\text{d}{\bf h}^\star \mathcal{O}({\bf h}, {\bf h}^\star) \,e^{S_{\rm loc}}
\end{equation}

\begin{equation}
    \alpha \frac{\partial Z_{\rm loc}}{\partial m_{kp}(a)} = -\int \mathcal{D}h\text{d}{\bf h}^\star  \,\left[\alpha h^\star_{p} \partial\ell({\bf h}^\star, {\bf h}(a) + {\bf h}^\star {\bf m}(a))_k\right]e^{S_{\rm loc}} = -\nu_{kp}(a)
\end{equation}
The second saddle point is a bit more complicated. Let's go back to $S_{\rm loc}$ before we integrated out $\hat{\bf h}$.

\begin{equation}
\begin{split}
    2 \alpha \frac{\partial Z_{\rm loc}}{\partial Q_{kh}(c,d)} &= \int \mathcal{D}h\mathcal{D}\hat{\bf h}\text{d}{\bf h}^\star  \,\frac{\partial}{\partial Q_{kh}(c,d)}\exp{\left\{\frac{1}{2}\int \text{d} a \text{d} b \, \hat{\bf h}(a)\hat{\bf h}(b){\bf Q}(a,b) + \int \text{d} a \, \hat{\bf h}(a){\bf h}(a) - \right.}\\&\qquad\qquad\qquad\qquad\qquad\qquad\qquad\qquad{\left. - \frac{1}{2}{\bf h}^{\star 2} - \int \text{d} a\, \ell({\bf h}^\star, {\bf h}(a) + {\bf h}^\star {\bf m}(a)) \right\}}\\
    &= \int \mathcal{D}h\mathcal{D}\hat{\bf h}\text{d}{\bf h}^\star  \, \hat{h}_k(c)\hat{h}_h(d)\exp{\left\{\frac{1}{2}\int \text{d} a \text{d} b \, \hat{\bf h}(a)\hat{\bf h}(b){\bf Q}(a,b) + \int \text{d} a \, \hat{\bf h}(a){\bf h}(a) - \right.}\\&\qquad\qquad\qquad\qquad\qquad\qquad\qquad\qquad{\left. - \frac{1}{2}{\bf h}^{\star 2} - \int \text{d} a\, \ell({\bf h}^\star, {\bf h}(a) + {\bf h}^\star {\bf m}(a)) \right\}}\\
   &= \int \mathcal{D}h\mathcal{D}\hat{\bf h}\text{d}{\bf h}^\star  \, \exp{\left\{\frac{1}{2}\int \text{d} a \text{d} b \, \hat{\bf h}(a)\hat{\bf h}(b){\bf Q}(a,b) - \int \text{d} a\, \ell({\bf h}^\star, {\bf h}(a) + {\bf h}^\star {\bf m}(a)) \right.}\\&\qquad\qquad\qquad\qquad\qquad\qquad\qquad\quad\,{\left. - \frac{1}{2}{\bf h}^{\star 2}\right\}\hat{h}_k(c)\hat{h}_h(d)  \exp{\left\{\int \text{d} a \, \hat{\bf h}(a){\bf h}(a)\right\}}}\\
   &= \int \mathcal{D}h\mathcal{D}\hat{\bf h}\text{d}{\bf h}^\star  \, \exp{\left\{\frac{1}{2}\int \text{d} a \text{d} b \, \hat{\bf h}(a)\hat{\bf h}(b){\bf Q}(a,b) - \int \text{d} a\, \ell({\bf h}^\star, {\bf h}(a) + {\bf h}^\star {\bf m}(a)) \right.}\\&\qquad\qquad\qquad\qquad\qquad\qquad\quad\,\,\,{\left. - \frac{1}{2}{\bf h}^{\star 2}\right\}\frac{\partial^2}{\partial {\bf h}(c)\partial {\bf h}(d)}  \exp{\left\{\int \text{d} a \, \hat{\bf h}(a){\bf h}(a)\right\}}}\\
   &= \int \mathcal{D}h\mathcal{D}\hat{\bf h}\text{d}{\bf h}^\star  \, \exp{\left\{\frac{1}{2}\int \text{d} a \text{d} b \, \hat{\bf h}(a)\hat{\bf h}(b){\bf Q}(a,b) + \int \text{d} a \, \hat{\bf h}(a){\bf h}(a)- \frac{1}{2}{\bf h}^{\star 2}\right\}}\\&\qquad\qquad\qquad\qquad\qquad\qquad\,\,{\frac{\partial^2}{\partial {\bf h}(c)\partial {\bf h}(d)}  \exp{\left\{-\int \text{d} a\, \ell({\bf h}^\star, {\bf h}(a) + {\bf h}^\star {\bf m}(a))\right\}}}\\
\end{split}
\end{equation}
In practice we first computed the variation with respect to ${\bf Q}$. This created ${\bf h}(c){\bf h}(d)$ in front of the exponential. Then, we wrote this as a double derivative with respect to $\hat{\bf h}$ of a piece in the action that "looks like an external field". Next, we realise that this is equivalent to taking the derivative with respect to ${\bf h}$ of the same piece. Finally, we integrate by part and obtain that we just need to take the derivative with respect to ${\bf h}$ of the loss term.
We now move forward:

\begin{equation}
    \frac{\partial}{\partial {h}_k(c)}e^{-\int \text{d} a\, \ell({\bf h}^\star, {\bf h}(a) + {\bf h}^\star {\bf m}(a))} = -\partial\ell({\bf h}^\star, {\bf h}(c) + {\bf h}^\star {\bf m}(c))_k\,e^{-\int \text{d} a\, \ell({\bf h}^\star, {\bf h}(a) + {\bf h}^\star {\bf m}(a))}
\end{equation}
and:

\begin{equation}
\begin{split}
    \frac{\partial^2}{\partial {h}_k(c){h}_h(d)}e^{-\int \text{d} a\, \ell({\bf h}^\star, {\bf h}(a) + {\bf h}^\star {\bf m}(a))} = \left[\partial\ell({\bf h}^\star, {\bf h}(c) + {\bf h}^\star {\bf m}(c))_k\partial\ell({\bf h}^\star, {\bf h}(d) + {\bf h}^\star m(d))_h \right.\\\left.- \delta(c,d)\partial^2 \ell({\bf h}^\star, {\bf h}(c) + {\bf h}^\star {\bf m}(c))_{kh}\right]\,e^{-\int \text{d} a\, \ell({\bf h}^\star, {\bf h}(a) + {\bf h}^\star {\bf m}(a))}
\end{split}
\end{equation}
In conclusion we have:

\begin{equation}
\begin{split}
    2 \alpha \frac{\partial Z_{\rm loc}}{\partial Q_{kh}(c,d)} = \alpha\llangle
    \partial\ell({\bf h}^\star, {\bf h}(c) + {\bf h}^\star {\bf m}(c))_k\partial\ell({\bf h}^\star, {\bf h}(d) + {\bf h}^\star m(d))_h\rrangle \\
    - \delta(c,d)\alpha\llangle\partial^2 \ell({\bf h}^\star, {\bf h}(c) + {\bf h}^\star {\bf m}(c))_{kh}\rrangle = {M}_{kh}(c,d) - \delta(c,d) {\bf \delta \lambda}_{kh}(d)
\end{split}
\end{equation}
The final form of the equations of motions is thus:

\begin{equation}
    \int \text{d}b \,\mathcal{K}(a,b) {\bf m}(b) = - {\bf \nu}(a)
\end{equation}
and:

\begin{equation}
    {\bf Q}^{-1}(a,b) = \mathcal{K}(a,b) - {\bf M}(a,b) + \delta(a,b){\bf \delta\lambda}(a)
\end{equation}
\subsection{Grassman identities and magnetisation}
There is still a lot of information that can be extracted from the theory we just derived. First, we will need some technical tools. We will define the Dirac delta for Grassman variables $\delta(a,b)$ as:
\begin{equation}
    \delta(a,b) = (\theta_a\hat\theta_a + \theta_b\hat\theta_b)\delta(t_a-t_b)
\end{equation}
We can show that with this definition we in fact have a delta function. Take any ${\bf m}(a)$, then:

\begin{equation}
\begin{split}
    \int \text{d} b\, \delta(a,b) {\bf m}(b) =& \int \text{d} b\, (\theta_a\hat\theta_a + \theta_b\hat\theta_b)\delta(t_a-t_b) (m(t_b) + \theta_b\bar\theta_b \hat m(t_b)) =\\
    =& \int \text{d} b\, \delta(t_a-t_b) (\theta_a\hat\theta_a m(t_b) + \theta_b\hat\theta_b m(t_b) + \theta_a\hat\theta_a\theta_b\hat\theta_b \hat m (t_b)) =\\
    =& \int \text{d} t_b\, \delta(t_a-t_b) (m(t_b) + \theta_a\hat\theta_a \hat m (t_b)) =\\
    =&\, m(t_a) + \theta_a\hat\theta_a \hat m (t_a) =\\
    =&\, {\bf m}(a)
\end{split}
\end{equation}
Next, we show that by by defining the operator $D(a,b)$:

\begin{equation}
    D(a,b) = - \theta_a\hat\theta_a \frac{\partial}{\partial t_a}\delta(t_b-t_a) - \theta_b\hat\theta_b \frac{\partial}{\partial t_b}\delta(t_a-t_b)
\end{equation}
we have the identity:
\begin{equation}
    \frac{1}{2}\int \text{d} a \text{d} b\, D(a,b) {\bf m}(a){\bf m}(b) = \int \text{d} t\, \hat m(t)\frac{\partial m(t)}{\partial t}
\end{equation}
This is proven by first noticing that:
\begin{equation}
\begin{split}
    \int \text{d} a \text{d} b\, \theta_a\hat\theta_a \frac{\partial}{\partial t_a}\delta(t_b-t_a) {\bf m}(a){\bf m}(b)= -\int \text{d} t_a \text{d} t_b\, \delta(t_b-t_a) \hat m(t_b)\frac{\partial m(t_a)}{\partial t_a} 
\end{split}
\end{equation}
and then symmetrising this expression.
Finally, recalling that:
\begin{equation}
    m^2(a) = m^2(t_a) + 2\theta_a\bar\theta_a m(t_a)\hat m(t_a)
\end{equation}
we have the explicit expression of the kernel $\mathcal{K}(a,b)$ as:

\begin{equation}
    \mathcal{K}(a,b) = D(a,b) + \lambda \delta(a,b)
\end{equation}
The equation of motion for ${\bf m}(a)$ can be rewritten as:

\begin{equation}
    \int \text{d}b \,D(a,b) {\bf m}(b) = - \lambda {\bf m}(a) - \nu(t)
\end{equation}
Now we make the time derivative explicit:

\begin{equation}
\begin{split}
    D(a,b){\bf m}(b) =& - \theta_a\bar\theta_a \frac{\partial}{\partial t_a}\delta(t_b-t_a){\bf m}(b) - \theta_b\bar\theta_b \frac{\partial}{\partial t_b}\delta(t_a-t_b){\bf m}(b) =\\
    =&\, \theta_a\bar\theta_a \delta(t_b-t_a)\frac{\partial {\bf m}(b)}{\partial t_a} + \theta_b\bar\theta_b \delta(t_a-t_b)\frac{\partial {\bf m}(b)}{\partial t_b} =\\
    =&\, \theta_b\bar\theta_b \delta(t_a-t_b)\left(\frac{\partial m(t_b)}{\partial t_b} + \theta_b\bar\theta_b\frac{\partial \hat m(t_b)}{\partial t_b}\right) =\\
    =&\, \theta_b\bar\theta_b \delta(t_a-t_b)\frac{\partial m(t_b)}{\partial t_b} \\
\end{split}
\end{equation}
so we have:
\begin{equation}
    \int \text{d}b \,D(a,b) {\bf m}(b) = \frac{\partial m(t_a)}{\partial t_a}
\end{equation}
Plugging this in the saddle point equation we obtain that $\hat m (t) = 0$ and:

\begin{equation}
    \frac{\partial m(t)}{\partial t} = - \lambda m(t) - \nu(t)
\end{equation}
\subsection{Self-consistent stochastic process}
We just need a way to compute the expectations $\llangle\cdot\rrangle$. This is not possible analytically as far as I know unless we are in really simple cases with linear activations and $\ell_2$ loss. We can however find a numerical procedure to study the equations. Let's plug in the second saddle point equation into $S_{\rm loc}$. We get:

\begin{equation}
\begin{split}
    S_{\rm loc} = -\frac{1}{2}\int \text{d} a \text{d} b \, {\bf h}(a){\bf h}(b)\mathcal{K}(a,b) + \frac{1}{2}\int \text{d} a \text{d} b \, {\bf h}(a){\bf h}(b)M(a,b) - \frac{1}{2} \int \text{d} a\, \delta\lambda(a) h^2(a) \\- \int \text{d} a\, \ell({\bf h}^\star, {\bf h}(a) + {\bf h}^\star m(t_a)) - \frac{1}{2}{\bf h}^{\star 2}     
\end{split}
\end{equation}
We want to show that this action is the MSR action for $h(t)$.
It's possible to show
%\cite{Kamenev_2011} 
that for any function $f(h)$:
\begin{equation}
    \llangle f(h(t))\hat{\bf h}(t) \rrangle = 0, \qquad \qquad \llangle f(h(t))f(h(t'))\hat{\bf h}(t)\hat{\bf h}(t') \rrangle = 0
\end{equation}
As a consequence we get that:

\begin{equation}
    M(a,b) = M_C(t_a,t_b) + \theta_a\bar\theta_a M_R(t_b,t_a)\theta(t_b-t_a) + \theta_b\bar\theta_b M_R(t_a,t_b)\theta(t_a-t_b)
\end{equation}
and:

\begin{equation}
    \delta\lambda(a) = \delta\lambda(t_a), \qquad\qquad \nu(a) = \nu(t_a)
\end{equation}
The indicator functions $\theta(t_b-t_a)$ are introduced to enforce causality in the theory.
We can now go back to the original time variables. We start with the kernel part, that by definition is:

\begin{equation}
    \frac{1}{2} \int \text{d} a \text{d} b\, \mathcal{K}(a,b) {\bf h}(a){\bf h}(b) = \int_0^{+\infty}\text{d} t \,\hat{\bf h}(t)\left( \frac{\partial h(t)}{\partial t} + \lambda h(t)\right)
\end{equation}
Next, the piece with $\delta \lambda$ will simplify as:

\begin{equation}
    \frac{1}{2}\int \text{d} a\, \delta\lambda(a) h^2(a) = \frac{1}{2}\int \text{d} a\, \delta\lambda(t_a) (h^2(t_a) + 2h(t_a)\hat{\bf h}(t_a) \theta_a\hat\theta_a) = \int_0^{+\infty} \text{d} t\, \delta\lambda(t) h(t)\hat{\bf h}(t)
\end{equation}
We can intuitively explain the computation above as follows. If you integrate any function of Grassman variables the only term that will survive is the piece that contains Grassman variables. In this case we have the product of multiple functions, so we need to pick the traditional variable part from all of them except one and sum over the possible choices. For the $M(a,b)$ term we get:

\begin{equation}
\begin{split}
    &\frac{1}{2}\int \text{d} a \text{d} b \, {\bf h}(a){\bf h}(b)M(a,b) =
    \frac{1}{2}\int \text{d} t_a \text{d} t_b h(t_a)\hat{\bf h}(t_b)  M_R(t_b,t_a)\theta(t_b-t_a)+ \\
    &\qquad+\frac{1}{2}\int \text{d} t_a \text{d} t_b h(t_b)\hat{\bf h}(t_a)  M_R(t_a,t_b)\theta(t_a-t_b) + \frac{1}{2}\int \text{d} t_a \text{d} t_b\hat{\bf h}(t_a)\hat{\bf h}(t_b)M_C(t_a,t_b) = \\
    &\qquad =\int \text{d} t_a \text{d} t_b h(t_b)\hat{\bf h}(t_a)  M_R(t_a,t_b)\theta(t_a-t_b) + \frac{1}{2}\int \text{d} t_a \text{d} t_b\hat{\bf h}(t_a)\hat{\bf h}(t_b)M_C(t_a,t_b) = \\
    &\qquad =\int_0^{+\infty} \text{d}t \hat{\bf h}(t) \int_0^t M_R(t,\tau)h(\tau) \text{d} \tau + \frac{1}{2}\int_0^{+\infty} \text{d} t \text{d} t'\hat{\bf h}(t)\hat{\bf h}(t')M_C(t,t')
\end{split}
\end{equation}
The motif is the same as the previous piece, with the additional complication of having both $\theta_a$ and $\theta_b$ to choose from. Finally we have the loss piece. For this we have:

\begin{equation}
    \int \text{d} a\, \ell({\bf h}^\star, {\bf h}(a) + {\bf h}^\star m(t_a)) = \int_0^{+\infty} \text{d}t\,\partial \ell({\bf h}^\star, h(t) + {\bf h}^\star m(t))\hat{\bf h} (t)
\end{equation}

Putting everything together we get:

\begin{equation}
\begin{split}
    S_{\rm loc} = \int_0^{+\infty}\text{d} t \,\hat{\bf h}(t)\left[ -\frac{\partial h(t)}{\partial t} - (\lambda+\delta\lambda(t)) h(t) - \partial \ell({\bf h}^\star, h(t) + {\bf h}^\star m(t)) + \int_0^t M_R(t,\tau)h(\tau) \text{d} \tau \right]\\ + \frac{1}{2}\int \text{d} t \text{d} t' \, \hat{\bf h}(t)\hat{\bf h}(t')M_C(t,t') - \frac{1}{2}{\bf h}^{\star 2}     
\end{split}
\end{equation}
As anticipated we this is in fact the MSR action of the following stochastic process for $h(t)$:

\begin{equation}
    \frac{\partial h(t)}{\partial t} = - \bar\lambda h(t) - \partial \ell({\bf h}^\star, h(t) + {\bf h}^\star m(t)) + \int_0^t M_R(t,\tau)h(\tau) \text{d} \tau + \xi
\end{equation}
with $\bar\lambda(t) = \lambda+\delta\lambda(t)$ and ${\bf h}^\star\sim\mathcal{N}(0,1)$ and:

\begin{equation}
    \langle \xi(t) \rangle = 0, \qquad\qquad \langle \xi(t)\xi(t') \rangle = M_C(t,t')
\end{equation}

This concludes the derivation of the DMFT.

\subsection{Staircase for Batch Gradient Descent (DMFT)}

We consider the case of squared loss.
Let $U^*$ denote the subspace spanned by ${\bf w^{\star}}^k$.
Suppose that at a given time $t$, the subspace learned by ${\bf w}_i^t$ is $U_t \subset U^*$.
We consider the projection of the gradient along a direction $\bf v\in U^*$ such that $\bf v \perp U_t $:

\begin{align*}
    \langle \nabla_{{\bf w}_t^k} \mathcal{L}_\nu, \bf v \rangle \approx  \frac{y_{\nu}}{\sqrt{K_S}}\sum_{k=1}^{K_S} u_k \phi'_{S}\left(\frac{{ {\bf w}_t^k}^\top \bf x_\nu}{\sqrt{d}}\right){\bf x_\nu}^\top {\bf v}
\end{align*}

We decompose ${\bf w}_t^k$ as ${{\bf w}^*_t}^k+{{\bf w}^\perp_t}^k$ where ${{\bf w}^*_t}^k \in U_t$ and ${{\bf w}^\perp_t}^k \perp  U^*$.

Assuming that $W^*{\bf w}_t^k$ i.e the overlap along the teacher concentrates,  $({{\bf w}^*_t}^k)^\top \bf x_\nu$ is Gaussian and independent of ${\bf x_\nu}^\top {\bf v}$. However, ${{\bf w}^\perp_t}^k$ depends on ${\bf v}$ and $({{\bf w}^\perp_t}^k)^\top {\bf v}$ can no longer assumed to be Gaussian.

\textcolor{blue}{Notice that if ${\bf v}^p$ is one of the vectors of the teacher, we have
\begin{equation}
    \langle \nabla_{{\bf w}_t^k} \mathcal{L}_\nu, {\bf v}^p \rangle \approx {\bf \nu}_{kp} = \alpha\llangle  h^\star_{p} \partial\ell({\bf h}^\star, {\bf h}(a) + {\bf h}^\star {\bf m}(a))_k \rrangle\,.
\end{equation}
This is as
\begin{equation}
    \mathcal{D}{\bf m}_{kp} = \langle \mathcal{D}{\bf w}_t^k \mathcal{L}_\nu, {\bf v}^p \rangle =\langle \nabla_{{\bf w}_t^k} \mathcal{L}_\nu, {\bf v}^p \rangle
\end{equation}
where $\mathcal{D}$ is the discrete derivative. On the other hand, when there is no weight decay ($\lambda = 0$)
\begin{equation}
    \mathcal{D}{\bf m}_{kp} = \nu_{kp}  \,  
\end{equation}
from which we have our identity.
PLEASE be careful with $h$, as we shifted it before equation (69)
}

\section{DMFT as in Gerbelot et al.}
{\bf FK: WHAT THE HECK IS THIS TITLE????}
Here we adapt Gerbelot et al. to this problem. First, we rewrite (informally) the results of theorem 3.2 with our notation. In the following we keep $P = 1$ while working in the limit of large input dimension $d\to\infty$ and the proportional regime $n = \alpha d$, with finite $\alpha$. Consider the $p$-th weight vector on the first later $\left(w^p\right)_i^\tau = W_{pi}^\tau$
%, its dicrete derviative $\left(v^p\right)^\tau_i = \left(w^p\right)^\tau_i-\left(w^p\right)^{\tau-1}_i $ 
and the preactivations of the $p$-th weight $\left(\lambda^p\right)^\nu$. In the large input limit we get that for all the $i$,
\begin{equation}
    \left(w^p\right)_i^\tau \to \left(\theta^p\right)^\tau
\end{equation}
%and 
%\begin{equation}
%    \left(v^p\right)_i^\tau \to \left(\nu^p\right)^\tau
%\end{equation}
Similarly, the preactivations converge for all $\nu$ as 
\begin{equation}
    \left(\lambda^p\right)^\nu \to r^p
\end{equation}

We will use the notation $\theta^p = {\boldsymbol{\theta}}$,
%, $v^p = {\boldsymbol{\nu}}$ 
$r^p = {\boldsymbol{r}}$ and consider all the implitic products as matrix-vector products. These new variables are defined by the following system of equations:
%\begin{equation}
%    \boldsymbol{\theta}^\tau = \sum_{t=0}^\tau %\boldsymbol{\nu}^t
%\end{equation}
\begin{equation}
    \boldsymbol{\theta}^{\tau+1} -  \boldsymbol{\theta}^\tau= -\alpha \,\eta\,\boldsymbol{\theta}^\tau \Lambda^\tau - \alpha\,\eta \sum_{t=0}^{\tau-1} \boldsymbol{\theta}^t R_\ell(\tau,t) + \sqrt{\alpha}\,\eta \boldsymbol{u}^\tau
\end{equation}
\begin{equation}
    \boldsymbol{r}^\tau = -\eta\sum_{t=0}^{\tau-1}\nabla_{\boldsymbol{r}} \mathcal{L}(\boldsymbol{r}^t) R_\theta(\tau,t) + \boldsymbol{\omega}^t
\end{equation}

Where we defined the random function $\ell:\mathbb{R}^p\to \mathbb{R}^p$ as the gradient of the loss with respect to the preactivations:
\begin{equation}
    s(\boldsymbol{r}) = \boldsymbol{a}\cdot \sigma{(\boldsymbol{r})} / \sqrt{p}
\end{equation}
\begin{equation}
    \mathcal{L}(\boldsymbol{r}) = \left(y - s(\boldsymbol{r})\right)^2/2
\end{equation}
\begin{equation}
    \mathcal{E}(\boldsymbol{r}) = y - s(\boldsymbol{r})
\end{equation}
\begin{equation}
    \ell(\boldsymbol{r}) = \nabla_{\boldsymbol{r}} \mathcal{L} = \mathcal{E}(\boldsymbol{r}) \,\boldsymbol{a}\cdot \nabla_{\boldsymbol{r}}\sigma{(\boldsymbol{r})} / \sqrt{p}
\end{equation}

and:
\begin{equation}
    \Lambda^\tau = \mathbb{E}\left[ \nabla_{\boldsymbol{r}}^2 \mathcal{L} (\boldsymbol{r}^\tau)\right]
\end{equation}
\begin{equation}
    R_\ell (\tau,t) = \mathbb{E}\left[ T_\ell(\tau,t) \right]
\end{equation}
\begin{equation}
    R_\theta (\tau,t) = \,\mathbb{E}\left[ T_\theta(\tau,t) \right]
\end{equation}
where:
\begin{equation}
     T_\ell(\tau,t) = \nabla_{\boldsymbol{r}}^2 \mathcal{L}(\boldsymbol{r}^\tau) \cdot \left( \sum_{s=t}^{\tau-1}R_\theta(\tau,s) T_\ell(s,t) +  R_\theta(\tau-1,t)\nabla_{\boldsymbol{r}}^2 \mathcal{L}(\boldsymbol{r}^t)\right)
\end{equation}
%\begin{equation}
%     T_\theta(\tau,t) = \sum_{s=0}^\tau T_\nu(s,t)
%\end{equation}
\begin{equation}
     T_\theta(\tau+1,t) - T_\theta(\tau,t) = T_\theta(\tau,t) \Lambda^\tau + \sum_{s=t}^{\tau-1}R_\ell(\tau,s)T_\theta(s,t)
\end{equation}
Finally, $\boldsymbol{u}^t$ and $\boldsymbol{\omega}^t$ are zero-mean Gaussian processes respectively with covariances $C_\ell(\tau,t)$ and $C_\theta(\tau,t)$:

\begin{equation}
    C_\ell(\tau,t) = \mathbb{E}\left[ \left(\boldsymbol{u}^\tau\right)^\top\boldsymbol{u}^t \right] = \mathbb{E}\left[ \nabla_{\boldsymbol{r}} \mathcal{L}(\boldsymbol{r}^\tau)^\top\nabla_{\boldsymbol{r}} \mathcal{L}(\boldsymbol{r}^t) \right]
\end{equation}
\begin{equation}
    C_\theta(\tau,t) = \mathbb{E}\left[ \left(\boldsymbol{\omega}^\tau\right)^\top\boldsymbol{\omega}^t \right] = \mathbb{E}\left[ \left(\boldsymbol{\theta}^\tau\right)^\top\boldsymbol{\theta}^t \right]
\end{equation}
Now we introduce the teacher. The equations become:
\begin{equation}
    \boldsymbol{\theta}^{\tau+1} -  \boldsymbol{\theta}^\tau= -\alpha \,\eta\,\boldsymbol{\theta}^\tau \Lambda^\tau - \alpha\,\eta\, R_\ell^*(\tau) \boldsymbol{\theta}^* - \alpha\,\eta \sum_{t=0}^{\tau-1} \boldsymbol{\theta}^t R_\ell(\tau,t) + \sqrt{\alpha}\,\eta\, \boldsymbol{u}^\tau
\end{equation}
\begin{equation}
    \boldsymbol{r}^\tau = -\eta\sum_{t=0}^{\tau-1}\nabla_{\boldsymbol{r}} \mathcal{L}(\boldsymbol{r}^t, \boldsymbol{r}^*) R_\theta(\tau,t) + \boldsymbol{\omega}^t
\end{equation}
%Where we defined the random function $\ell:\mathbb{R}^p\to \mathbb{R}^p$ as the %gradient of the loss with respect to the preactivations:
%\begin{equation}
%    s(\boldsymbol{r}) = \boldsymbol{a}\cdot \sigma{(\boldsymbol{r})} / \sqrt{p}
%\end{equation}
%\begin{equation}
%    \mathcal{L}(\boldsymbol{r}) = \left(y - s(\boldsymbol{r})\right)^2/2
%\end{equation}
%\begin{equation}
%    \mathcal{E}(\boldsymbol{r}) = y - s(\boldsymbol{r})
%\end{equation}
%\begin{equation}
%    \ell(\boldsymbol{r}) = \nabla_{\boldsymbol{r}} \mathcal{L} = 
%\end{equation}

and:
\begin{equation}
    \Lambda^\tau = \mathbb{E}\left[ \nabla_{\boldsymbol{r}}^2 \mathcal{L} (\boldsymbol{r}^\tau, \boldsymbol{r}^*)\right]
\end{equation}
\begin{equation}
    R_\ell^* (\tau) = \mathbb{E}\left[ T_\ell^*(\tau) \right]
\end{equation}
\begin{equation}
    R_\ell (\tau,t) = \mathbb{E}\left[ T_\ell(\tau,t) \right]
\end{equation}
\begin{equation}
    R_\theta (\tau,t) = \,\mathbb{E}\left[ T_\theta(\tau,t) \right]
\end{equation}
where:
\begin{equation}
    T_\ell^*(\tau) = \nabla_{\boldsymbol{r}}^2 \mathcal{L}(\boldsymbol{r}^\tau, \boldsymbol{r}^*) \cdot  \sum_{s=t}^{\tau-1}R_\theta(\tau,s) T_\ell^*(s) + \nabla_{\boldsymbol{r}}\nabla_{\boldsymbol{r}^*} \mathcal{L}(\boldsymbol{r}^\tau, \boldsymbol{r}^*)
\end{equation}
\begin{equation}
     T_\ell(\tau,t) = \nabla_{\boldsymbol{r}}^2 \mathcal{L}(\boldsymbol{r}^\tau, \boldsymbol{r}^*) \cdot \left( \sum_{s=t}^{\tau-1}R_\theta(\tau,s) T_\ell(s,t) +  R_\theta(\tau,t)\nabla_{\boldsymbol{r}}^2 \mathcal{L}(\boldsymbol{r}^t, \boldsymbol{r}^*)\right)
\end{equation}
%\begin{equation}
%     T_\theta(\tau,t) = \sum_{s=0}^\tau T_\nu(s,t)
%\end{equation}
\begin{equation}
     T_\theta(\tau+1,t) - T_\theta(\tau,t) = T_\theta(\tau,t) \Lambda^\tau + \sum_{s=t}^{\tau-1}R_\ell(\tau,s)T_\theta(s,t)
\end{equation}
Finally, $\boldsymbol{u}^t$ and $\boldsymbol{\omega}^t$ are zero-mean Gaussian processes respectively with covariances $C_\ell(\tau,t)$ and $C_\theta(\tau,t)$:

\begin{equation}
    C_\ell(\tau,t) = \mathbb{E}\left[ \left(\boldsymbol{u}^\tau\right)^\top\boldsymbol{u}^t \right] = \mathbb{E}\left[ \nabla_{\boldsymbol{r}} \mathcal{L}(\boldsymbol{r}^\tau)^\top\nabla_{\boldsymbol{r}} \mathcal{L}(\boldsymbol{r}^t) \right]
\end{equation}
\begin{equation}
    C_\theta(\tau,t) = \mathbb{E}\left[ \left(\boldsymbol{\omega}^\tau\right)^\top\boldsymbol{\omega}^t \right] = \mathbb{E}\left[ \left(\boldsymbol{\theta}^\tau\right)^\top\boldsymbol{\theta}^t \right]
\end{equation}

\textcolor{blue}{I don't remember the exact manipulations but you get that}
\begin{equation}
    M^\tau = \mathbb{E}\left[ \left(\boldsymbol{\theta}^\tau\right)^\top \boldsymbol{\theta}^*\right]
\end{equation}
which obeys the equation:
\begin{equation}
    M^{\tau + 1} - M^{\tau} = \alpha\,\eta\,\mathbb{E}\left[ \nabla_{\boldsymbol{r}} \mathcal{L}(\boldsymbol{r}^\tau, \boldsymbol{r}^*) (\boldsymbol{r}^*)^\top\right]
\end{equation}
You can then decompose $\boldsymbol{r}^\tau$ into a component in the teacher subspace and one in the student subspace:
\begin{equation}
    \boldsymbol{r}^\tau = \boldsymbol{r}^\tau_\perp + M^\tau \boldsymbol{r}^*
\end{equation}
with the new equation:
\begin{equation}
    \boldsymbol{r}^{\tau+1}_\perp -  \boldsymbol{r}^\tau_\perp= -\alpha \,\eta\,\boldsymbol{r}^\tau_\perp \Lambda^\tau - \eta\,\nabla_{\boldsymbol{r}} \mathcal{L}(\boldsymbol{r}^t, \boldsymbol{r}^*) - \alpha\,\eta \sum_{t=0}^{\tau-1} \boldsymbol{r}^t_\perp R_\ell(\tau,t) + \sqrt{\alpha}\,\eta\, \boldsymbol{u}^\tau
\end{equation}
I believe from this we can see a staircase phenomenon: we start with $M^0 = 0$, so $\boldsymbol{r}^\tau = \boldsymbol{r}^\tau_\perp$. Then, at the first step you will (hopefully) get $\left(M^1\right)_{p1} \neq 0$ and $\boldsymbol{r}^\tau$ will get a spike and so on.
