# Supplementary material for: The Benefits of Reusing Batches for Gradient Descent in Two-Layer Networks: Breaking the Curse of Information and Leap Exponents
Source: arXiv:2402.03220 source file (2024-06-30)
Supplement: Supplementary file 2 [file saad-solla.tex]

\section{Online Gradient Descent Analysis}
\label{sec:app:saad_solla}\
\lp{WIP: adapt the section to novel findings, please ignore at present time.}
In this section we discuss the exact asymptotics analysis of online gradient descent in the proportional batch size regime $\alpha = \frac{n}{d} = O(1)$. Similar to the DMFT approach, we describe the low-dimensional process of the overlap matrices. However, without the re-use of the same batch multiple times, we are able to describe an Ordinary Differential Equations (ODE) for the process. 
\dots 
